# Supplementary material for: Tuning the Selective Permeability of Polydisperse Polymer Networks
Source: arXiv:2004.09175 source file (2020-04-20)
Supplement: Supplementary file 1 [file SI.pdf]

# Supplementary Information:
# Tuning the Selective Permeability of Polydisperse Polymer Networks

Won Kyu Kim,[1,*] Richard Chudoba,[2,3] Sebastian Milster,[2,4]
Rafael Roa,[5] Matej Kanduč,[6] and Joachim Dzubiella[2,4,7,†]

[1] *Korea Institute for Advanced Study, Seoul 02455, Republic of Korea*
[2] *Research Group for Simulations of Energy Materials, Helmholtz-Zentrum Berlin für Materialien und Energie, D-14109 Berlin, Germany*
[3] *Division of Theoretical Chemistry, Department of Chemistry, Lund University, P.O. Box 124, SE-22100 Lund, Sweden*
[4] *Applied Theoretical Physics-Computational Physics, Physikalisches Institut, Albert-Ludwigs-Universität Freiburg, D-79104 Freiburg, Germany*
[5] *Departamento de Física Aplicada I, Facultad de Ciencias, Universidad de Málaga, E-29071 Málaga, Spain*
[6] *Jožef Stefan Institute, SI-1000 Ljubljana, Slovenia*
[7] *Cluster of Excellence livMatS @ FIT - Freiburg Center for Interactive Materials and Bioinspired Technologies, Albert-Ludwigs-Universität Freiburg, D-79110 Freiburg, Germany*

## I. COMPUTER SIMULATIONS AND SUPPORTING RESULTS

### A. Cross-linker radial distribution functions

We show in Fig. S1 the two-dimensional radial distribution function $g_{\rm xx}^{\rm 2D}(r)$ between cross-linkers (x) in the network for different values of $\phi_{\rm n}$ and $\epsilon_{\rm np}$. Due to the slab geometry, the pair correlation functions were computed from averaging within thin membrane slabs (of thickness $1\sigma$) in $xy$-directions, and finally averaged over all slabs. The number of the membrane slabs ranges from 18 to 38, depending on the whole membrane width (see Fig. S3).

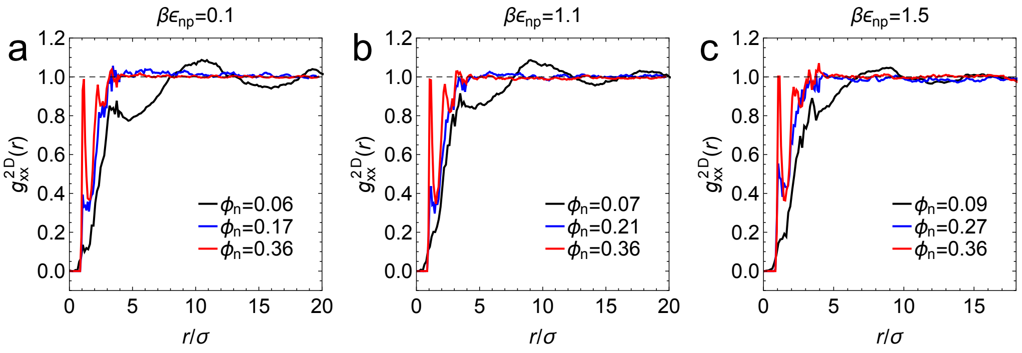


FIG. S1. Two-dimensional radial distribution functions $g_{\rm xx}(r)$ between the cross-linkers for different values of $\phi_{\rm n}$ and $\epsilon_{\rm np}$.

### B. Virial coefficients for partitioning

In Table S1 we show the virial coefficients $B_2^{\rm np}$ and $B_3^{\rm nnp}$ obtained from fitting the partitioning $\mathcal{K}(\phi_{\rm n})$ in Fig. 3a in the main text by the virial expression eqn (2) in the main text.

We show in Fig. S2a the fitted second virial coefficients $B_2^{\rm np}$ in Table S1 (symbols) in comparison with $B_2$ (solid curve) for the LJ interaction:

$$B_2(\epsilon_{\rm np}) = \int_0^\infty {\rm d}r 2\pi r^2 [1 - \exp(-\beta U_{\rm LJ}^{\rm np}(r, \epsilon_{\rm np}))], \tag{S1}$$

* wonkyukim@kias.re.kr
† joachim.dzubiella@physik.uni-freiburg.de

TABLE S1. Virial coefficients $B_2^{\mathrm{np}}$ and $B_3^{\mathrm{nnp}}$ in eqn (2) obtained as fitting parameters in Fig. 3a in the main text.

| $\beta\epsilon_{\mathrm{np}}$ | 0.1 | 0.7 | 1.0 | 1.1 | 1.2 | 1.5 |
|---|---|---|---|---|---|---|
| $B_2^{\mathrm{np}}/\sigma^3$ | $0.63 \pm 0.08$ | $-2.25 \pm 0.17$ | $-4.82 \pm 0.19$ | $-5.61 \pm 0.16$ | $-6.52 \pm 0.21$ | $-9.26 \pm 0.34$ |
| $B_3^{\mathrm{nnp}}/\sigma^6$ | $3.85 \pm 0.35$ | $4.74 \pm 0.44$ | $6.85 \pm 0.45$ | $7.46 \pm 0.38$ | $8.31 \pm 0.48$ | $10.41 \pm 0.74$ |

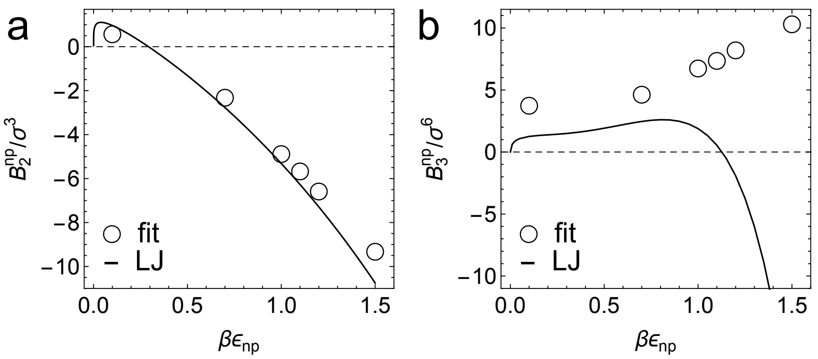


FIG. S2. (a) The fitted second virial coefficients $B_2^{\mathrm{np}}$ in Table S1 (symbols) are compared with $B_2$ (solid curve) for the LJ interaction. (b) The fitted third virial coefficients $B_3^{\mathrm{np}}$ in Table S1 (symbols) are compared with $B_3$ (solid curve) for the LJ interaction.

where we use the length parameter $\sigma_{\mathrm{nn}} = \sigma_{\mathrm{np}} = \sigma$.

In a similar manner we show in Fig. S2b the fitted third virial coefficients $B_3^{\mathrm{np}}$ in Table S1 (symbols) in comparison with $B_3$ (solid curve) for the one-component LJ interaction:

$$B_3(\epsilon) = -\frac{1}{3}\int_{\mathcal{V}}\int_{\mathcal{V}} \mathrm{d}^3\mathbf{r}_{12}\mathrm{d}^3\mathbf{r}_{13}[1-\exp(-\beta U_{\mathrm{LJ}}(r_{12},\epsilon))][1-\exp(-\beta U_{\mathrm{LJ}}(r_{13},\epsilon))][1-\exp(-\beta U_{\mathrm{LJ}}(r_{23},\epsilon))], \quad \text{(S2)}$$

where $\mathcal{V}$ is the total volume.

### C. Mean concentration profiles of networks and penetrants

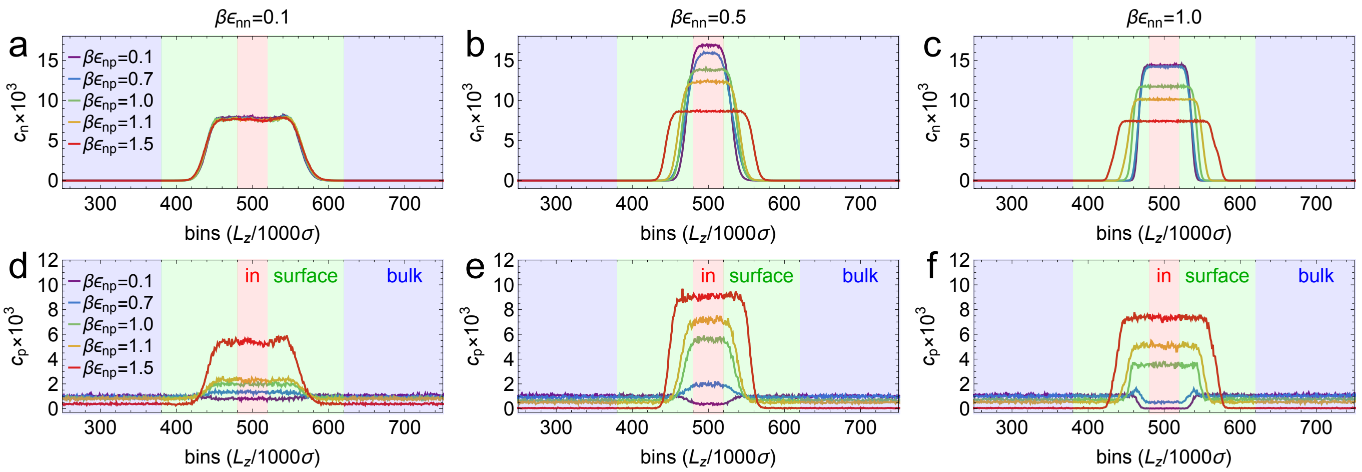


FIG. S3. Upper panels: network monomer concentration $c_{\mathrm{n}}(z)$ in a good ((a) $\beta\epsilon_{\mathrm{nn}} = 0.1$), intermediate ((c) $\beta\epsilon_{\mathrm{nn}} = 0.5$), and poor solvent ((c) $\beta\epsilon_{\mathrm{nn}} = 1.0$) with different network–penetrant interactions $\beta\epsilon_{\mathrm{np}}$. Lower panels: penetrant concentration $c_{\mathrm{p}}(z)$ in (d) the good, (e) intermediate, and (f) poor solvent with different network–penetrant interactions $\beta\epsilon_{\mathrm{np}}$. Three regions (in, surface, and bulk) are depicted in each plot by different colors, where we sampled the partitioning in the region "in".

We show in Fig. S3 the mean concentration profiles of the polymer network monomers and the penetrants in the

longitudinal direction $z$. The upper panels depict the network monomer concentration $c_{\rm n}(z)$ in a good ($\beta\epsilon_{\rm nn} = 0.1$), intermediate ($\beta\epsilon_{\rm nn} = 0.5$), and poor solvent ($\beta\epsilon_{\rm nn} = 1.0$) with different network–penetrant attractions $\beta\epsilon_{\rm np}$. The lower panels depict the penetrant concentration $c_{\rm p}(z)$ in the good ($\beta\epsilon_{\rm nn} = 0.1$), intermediate ($\beta\epsilon_{\rm nn} = 0.5$), and poor solvent ($\beta\epsilon_{\rm nn} = 1.0$) with different network–penetrant attractions $\beta\epsilon_{\rm np}$. We show three regions (in, surface, and bulk) by different colors in each plot, where we sampled the partitioning in the region "in".

### D. Calculations for diffusivity inside the network

To calculate the penetrant diffusivity in the membrane, $D_{\rm in}$, we generated 20 simulation set ups with 3D periodic boundary conditions of the polydisperse tetra-functional networks including the penetrants for each parameter set of $\epsilon_{\rm nn}$ and $\epsilon_{\rm np}$, as shown in Fig. S4. To determine the cubic box size and the number of the penetrants in the cell, we used the equilibrium values of the penetrant density and the polymer density obtained from the main simulation data from the anisotropic setups. We carried out the simulations typically for $10^4$ time steps. We computed the mean-squared-displacement (MSD) of the penetrants in the networks, averaged over time and particles [1], as shown in Fig. S5 (upper panels), within the dimensionless simulation time range from $t = 100$ to $t = 1000$ to obtain diffusivity via MSD $= 6D_{\rm in}t$, ensuring the normal diffusion [1], which fulfills $\alpha = \frac{{\rm d}\ln{\rm MSD}}{{\rm d}\ln t} = 1$ in Fig. S5 (lower panels).

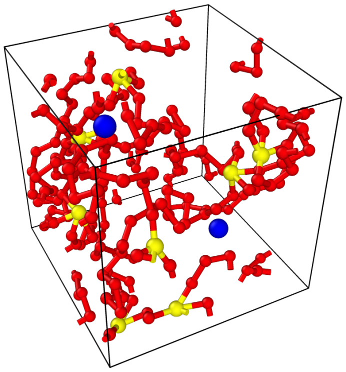

FIG. S4. Simulation snapshot of the polydisperse tetra-functional network with penetrants (blue) used to calculate the penetrant diffusivity $D_{\rm in}$.

### E. Network (slab membrane) volume

In Fig. S6 we show the network slab volume $V_{\rm n}$ as a function of the solvent quality $\epsilon_{\rm nn}$. As $\epsilon_{\rm nn}$ increases the volume decays rapidly until around $\epsilon_{\rm nn} = 0.5\ k_{\rm B}T$. As the network–penetrant interaction energy $\epsilon_{\rm np}$ increases up to $\epsilon_{\rm np} = 1.5\ k_{\rm B}T$, the volume considerably decreases, indicating the onset of the penetrant-induced collapse [2]. We calculate the polymer volume fraction using $\phi_{\rm n} = (N_{\rm m} + N_{\rm x})v_0/V_{\rm n}$, where $v_0 = \pi\sigma^3/6$ is the monomer volume with the diameter $\sigma = \sigma_{\rm nn} = \sigma_{\rm np}$.

### F. Scaling theories for the penetrant diffusivity

In Fig. S7 we compare the simulation results (symbols) with various scaling theories (solid curves) for the penetrant diffusivity in the polymer networks. In Fig. S7a we show the free-volume theory [3–9]

$$D_{\rm in}/D_0 = b{\rm e}^{-c\left(\frac{\phi_{\rm n}}{1-\phi_{\rm n}}\right)}. \tag{S3}$$

In Fig. S7b we show the hydrodynamic/obstruction theory [9, 10]

$$D_{\rm in}/D_0 = {\rm e}^{-a(\phi_{\rm n})^{\nu}}. \tag{S4}$$

In Fig. S7c we show the extended barrier-crossing theory [11, 12]

$$D_{\rm in}/D_0 = \frac{1}{1+\alpha{\rm e}^{\beta\epsilon_{\rm np}}\left(\phi_{\rm n}\right)^{\zeta}}. \tag{S5}$$

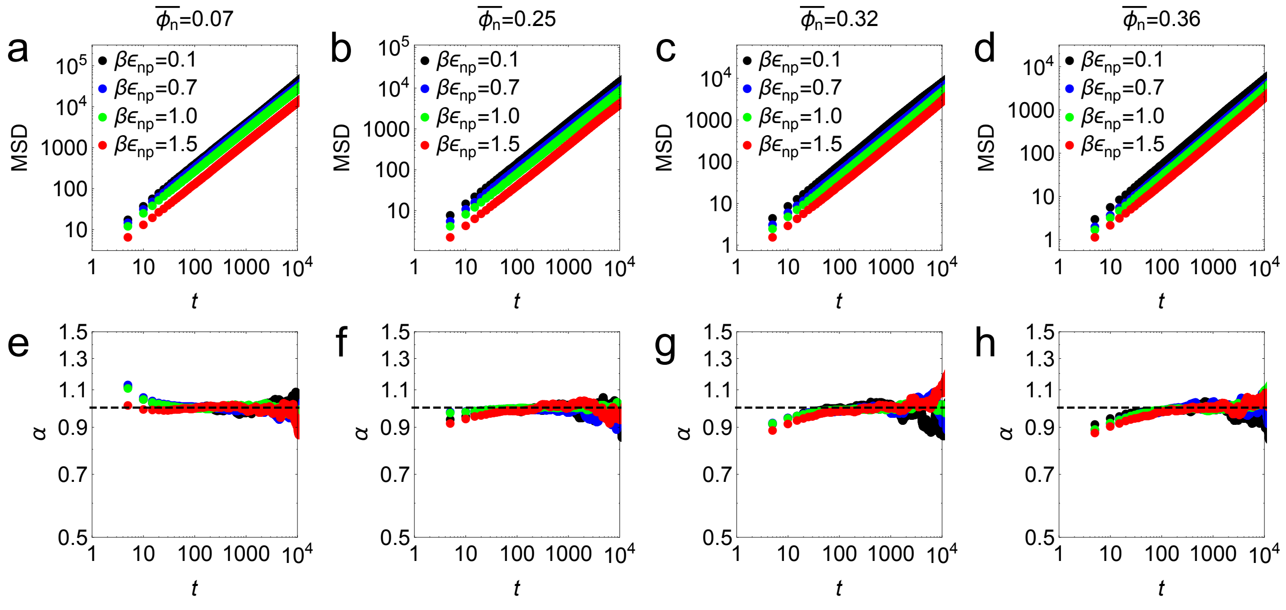


FIG. S5. Upper panels: Mean-squared-displacement (MSD($t$)) of the penetrants in the networks. Lower panels: The exponent $\alpha$ in MSD($t$) $\sim t^{\alpha}$.

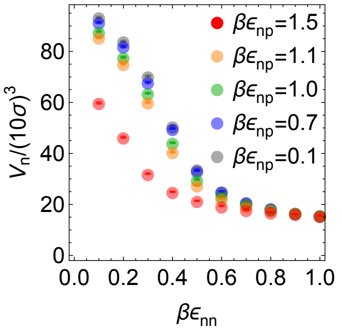


FIG. S6. Total network (slab) volume $V_{\mathrm{n}}$ as a function of the solvent quality $\epsilon_{\mathrm{nn}}$ for different values of the network–penetrant interaction $\epsilon_{\mathrm{np}}$.

In Fig. S7d we show the barrier-crossing theory [12, 13]

$$D_{\mathrm{in}}/D_0 = \xi \mathrm{e}^{-\beta\epsilon_{\mathrm{np}}} \left(\phi_{\mathrm{n}}\right)^{-\lambda}. \tag{S6}$$

All the fitting parameters are shown in Table S2, and in Fig. S8 we show the parameters $b$ and $c$ for the free-volume theory, $D_{\mathrm{in}}/D_0 = b\mathrm{e}^{-c\left(\frac{\phi_{\mathrm{n}}}{1-\phi_{\mathrm{n}}}\right)}$ from eqn S3. We note that $b$ is an exponentially decreasing function of $\epsilon_{\mathrm{np}}$, while $c$ is rather independent of $\epsilon_{\mathrm{np}}$, which leads to our scaling expression for the penetrant diffusivity,

$$D_{\mathrm{in}}/D_0 \sim \mathrm{e}^{-\beta\epsilon_{\mathrm{np}} - c\left(\frac{\phi_{\mathrm{n}}}{1-\phi_{\mathrm{n}}}\right)}. \tag{S7}$$

### G. Partitioning and mean penetrant number inside the network for large attractions

In Figs. S9a and b, the partitioning $\log_{10}\mathcal{K}$ is shown vs. $\epsilon_{\mathrm{nn}}$ and $\phi_{\mathrm{n}}$ for various interaction strengths, ranging from low $\epsilon_{\mathrm{np}} = 0.1\ k_{\mathrm{B}}T$ to high $\epsilon_{\mathrm{np}} = 2\ k_{\mathrm{B}}T$. For large network–penetrant attraction and dense packing, simulation results become noisy. This is due to strong confinement effects which result in nonequilibrium metastable states. In Fig. S9c we show the mean penetrant number $n_{\mathrm{in}}$ per unit volume $v \equiv V(\epsilon_{\mathrm{nn}}, \epsilon_{\mathrm{np}})/1000$ inside the network, which is also maximized with respect to $\phi_{\mathrm{n}}$. The mean penetrant number $n_0$ per $v$ outside the network, on the other hand, shown in Fig. S9d, is minimized with respect to $\phi_{\mathrm{n}}$.

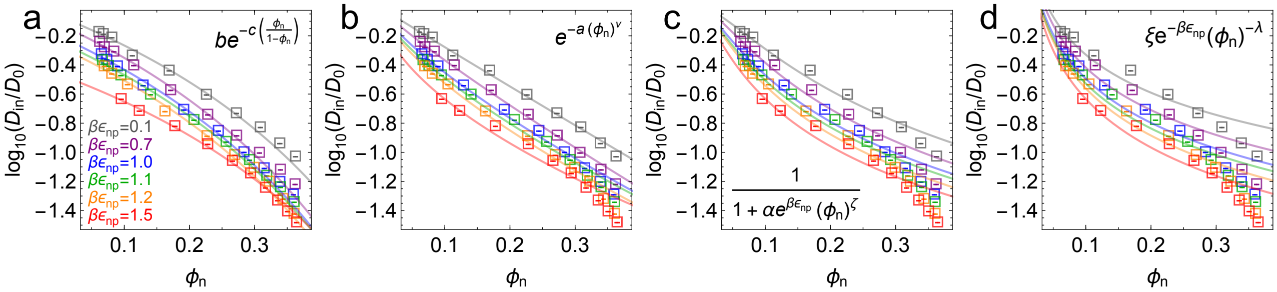


FIG. S7. Penetrant diffusivity in polymer networks compared with various scaling theories. (a) Free-volume theory (as shown in the main text), (b) hydrodynamic/obstruction theory, (c) extended barrier-crossing theory, (d) barrier-crossing theory. See Table S2 for the fitting parameters.

TABLE S2. Parameters in the scaling theories shown in Fig. S7, fitted from the simulation data.

| $\beta\epsilon_{np}$ | 0.1 | 0.7 | 1.0 | 1.1 | 1.2 | 1.5 |
|---|---|---|---|---|---|---|
| $b$ | $0.86 \pm 0.02$ | $0.76 \pm 0.02$ | $0.63 \pm 0.02$ | $0.57 \pm 0.01$ | $0.53 \pm 0.02$ | $0.34 \pm 0.01$ |
| $c$ | $4.17 \pm 0.19$ | $4.81 \pm 0.16$ | $4.77 \pm 0.19$ | $4.69 \pm 0.18$ | $4.79 \pm 0.20$ | $3.87 \pm 0.09$ |
| $a$ | $6.10 \pm 0.30$ | $6.43 \pm 0.23$ | $5.98 \pm 0.22$ | $5.83 \pm 0.23$ | $5.96 \pm 0.22$ | $5.35 \pm 0.35$ |
| $\nu$ | $0.98 \pm 0.03$ | $0.88 \pm 0.02$ | $0.76 \pm 0.02$ | $0.71 \pm 0.02$ | $0.69 \pm 0.02$ | $0.56 \pm 0.04$ |
| $\alpha$ | $29.71 \pm 4.51$ | $22.55 \pm 4.07$ | $18.21 \pm 3.13$ | $17.35 \pm 3.06$ | $18.42 \pm 3.15$ | $14.61 \pm 3.21$ |
| $\zeta$ | $1.54 \pm 0.07$ | $1.50 \pm 0.08$ | $1.40 \pm 0.07$ | $1.37 \pm 0.08$ | $1.39 \pm 0.07$ | $1.30 \pm 0.11$ |
| $\xi$ | $0.07 \pm 0.01$ | $0.08 \pm 0.02$ | $0.09 \pm 0.02$ | $0.08 \pm 0.02$ | $0.08 \pm 0.01$ | $0.08 \pm 0.02$ |
| $\lambda$ | $0.87 \pm 0.08$ | $0.97 \pm 0.09$ | $1.01 \pm 0.08$ | $1.02 \pm 0.08$ | $1.08 \pm 0.08$ | $1.11 \pm 0.11$ |

### H. Effects of different penetrant bulk concentrations

In Fig. S10 we show the effect of penetrant concentration on the partitioning. Upon increasing the penetrant number $N_p$ by two times, the partitioning with the low attraction $\beta\epsilon_{np} = 0.1$ becomes larger as the network volume fraction $\phi_n$ increases, while it becomes smaller with the large attraction $\beta\epsilon_{np} = 1.5$. However, an overall characteristic behavior of the partitioning remains robust.

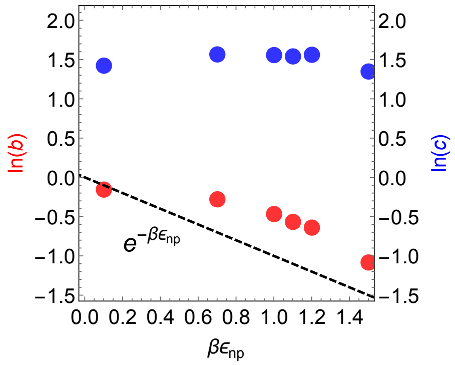

FIG. S8. Parameters $b$ (red, lower symbols) and $c$ (blue, upper symbols) shown in Table S2 for the free-volume theory $D_{\rm in}/D_0 = b e^{-c\left(\frac{\phi_{\rm n}}{1-\phi_{\rm n}}\right)}$ from eqn S3.

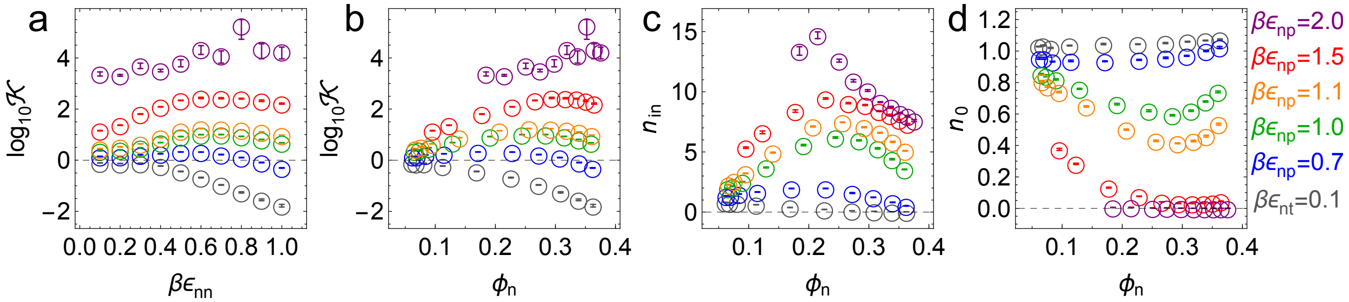

FIG. S9. Partitioning $\log_{10}\mathcal{K}$ as a function of (a) $\epsilon_{\rm nn}$ and (b) $\phi_{\rm n}$, up to a high attraction of $\epsilon_{\rm np} = 2\ k_{\rm B}T$. (c) Mean penetrant number $n_{\rm in}$ per unit volume inside the network as a function of the volume fraction $\phi_{\rm n}$. (d) Mean penetrant number $n_0$ per unit volume outside the network, as a function of the polymer volume fraction $\phi_{\rm n}$.

## II. COARSE-GRAINING OF POLYMER BOND PARAMETERS FROM ALL-ATOM SIMULATIONS

To obtain the parameters for the bonded potentials in our computer simulations, we used all-atom simulation setups of poly($N$-isopropylacrylamide) (PNIPAM) chains crosslinked by $N,N'$-methylenebisacrylamide (BIS), embedded in water at 290 K, from previous work [14] and as shown in Fig. S11. In particular, we set up two different systems. The first one comprises a BIS cross-linker with four PNIPAM monomers, *i.e.*, each BIS' backbone binding site is terminated by one monomer. This system enables the study of the conformations of PNIPAM chains attached to the cross-linker. The second system consist of a single PNIPAM trimer in water and is used to retrieve the bonding and bending information of the polymer chains only.

### A. All-atom simulation details

We employed explicit-water, all-atom molecular dynamics simulations with the OPLS-based force-field developed in Refs. [14] and [15] for the aforementioned systems. Twelve different initial configurations of the BIS-PNIPAM molecule were placed in individial cubic boxes (box length $\approx 4$ nm) with approximately 6500 water molecules. For the PNIPAM trimer we created 17 replicas, each solvated in a box (box length $\approx 2.5$ nm) of around 1500 water molecules.

After the initial energy minimization (steepest descent), the system was equilibrated in the $NVT$ ensemble for 2 ns and in the $NpT$ ensemble for an additional 2 ns. The integration step of the leap-frog integrator was set to 2 fs and data were collected every 1 ps during a production simulation time of 100 ns.

The linear constraint solver algorithm [16] was used for all hydrogen bonds, and the SPC/E force field was used for water molecules. We considered cut-off lengths for LJ and short-range electrostatic interactions as 1 nm. The particle mesh Ewald method with cubic interpolation with a grid spacing of 0.12 nm was used for long-range electrostatics [17]. We used periodic boundary conditions in all three Cartesian directions. The temperature and the pressure in the simulations were controlled by the velocity-rescale thermostat (at temperature $T = 290$ K and the relaxation time

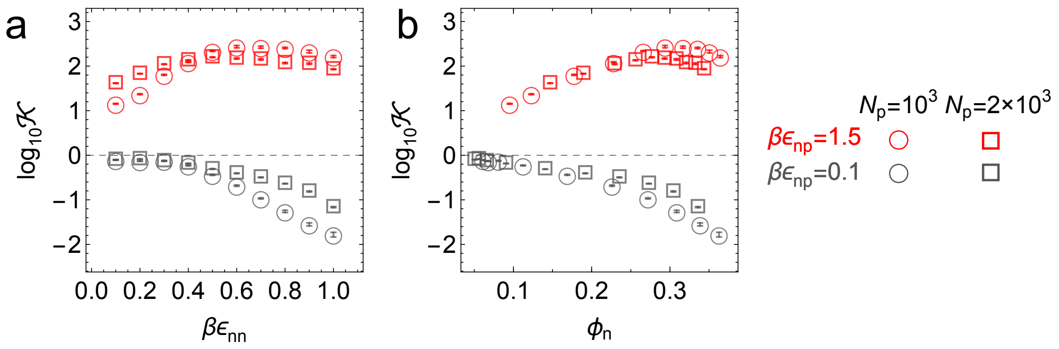


FIG. S10. Effects of different penetrant concentrations on the partitioning $\log_{10}\mathcal{K}$ vs. (a) $\epsilon_{\rm nn}$ and (b) $\phi_{\rm n}$ for the different total number of penetrants, $N_{\rm p} = 10^3$ (circles) and $N_{\rm p} = 2 \times 10^3$ (rectagles), and for the network–penetrant interaction values of $\beta\epsilon_{\rm np} = 0.1$ (gray) and $\beta\epsilon_{\rm np} = 1.5$ (red).

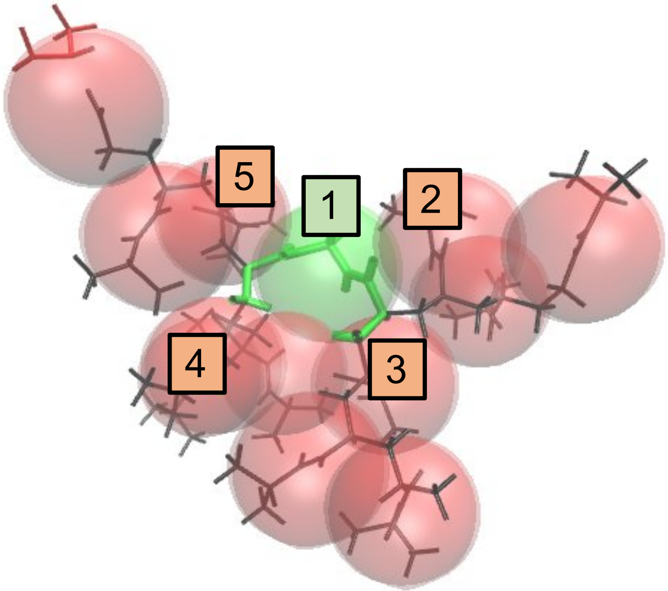


FIG. S11. Illustration of an all-atom and its corresponding coarse-grained (CG) representation of PNIPAM–BIS (poly($N$-isopropylacrylamide)–$N,N'$-methylenebisacrylamide), *i.e.*, one cross-linker and four attached chains with three monomers each. The spheres represent the coarse-grained beads located at the (all-atom) monomers' centers of masses for one cross-linker (green) and the chain (red). In order to obtain the bond potential parameters used in the main work, two minimal systems were simulated on the all-atom level with explicit water (not shown) at 290 K. The first one consists of one cross-linker (labeled 1) with four PNIPAM monomers (labeled 2, 3, 4, 5), the other one investigates a single PNIPAM trimer.

constant $\tau_T = 0.1$ ps) and the Berendsen barostat (at pressure $p = 1$ bar and the relaxation time constant $\tau_p = 1$ ps), respectively [18, 19].

### B. Bond parameters for the polymer networks

In our simulations of the polymer network we considered two-body (stretching) and three-body (bending) bond potentials, which are approximated as harmonic interactions,

$$F_r^{ij}(r^{ij}) = K_r^{ij}(r^{ij} - r_0^{ij})^2, \tag{S8}$$

$$F_\theta^{ijk}(\theta^{ijk}) = K_\theta^{ijk}(\theta^{ijk} - \theta_0^{ijk})^2, \tag{S9}$$

where $i, j, k =$ m or x is the particle index with m for the PNIPAM monomer and x for the BIS cross-linker. There are two stretching potentials $F_r^{\rm mm}$ and $F_r^{\rm mx}$, and since the BIS connects four PNIPAM chains (*i.e.*, tetra-functional) there are six bending potentials in $F_\theta^{\rm mxm}$ and one bending potential in $F_\theta^{\rm mmm}$. Therefore, we have nine different bond potentials in total and we determine eighteen bond parameters $K_r^{ij}$, $r_0^{ij}$, $K_\theta^{ijk}$, and $\theta_0^{ijk}$ by fitting to the free energies obtained from the all-atom simulations.

In Fig. S12 the symbols show the free energies $F_r$ and $F_\theta$ evaluated from the all-atom simulations, and the solid curves depict the harmonic potentials shown in eqns S8 and S9 with fitted parameters (see Table S3). For analyses we used 12 production trajectories of the PNIPAM–BIS simulations, and 17 production trajectories of the PNIPAM simulations, respectively. The six different bending free energies $F_\theta^{\rm mxm}$ at the BIS cross-linker are shown from Figs. S12a to f. These $F_\theta^{\rm mxm}$ have three complementary pairs due to the tetra-functional geometry as shown in Fig. S11. We show these three pairs of the bending free energy in Figs. S12a and b for 2-1-3 and 4-1-5 CG monomers, Figs. S12c and d for 2-1-5 and 3-1-4 CG monomers, Figs. S12e and f for 2-1-4 and 3-1-5 CG monomers, respectively. The stretching free

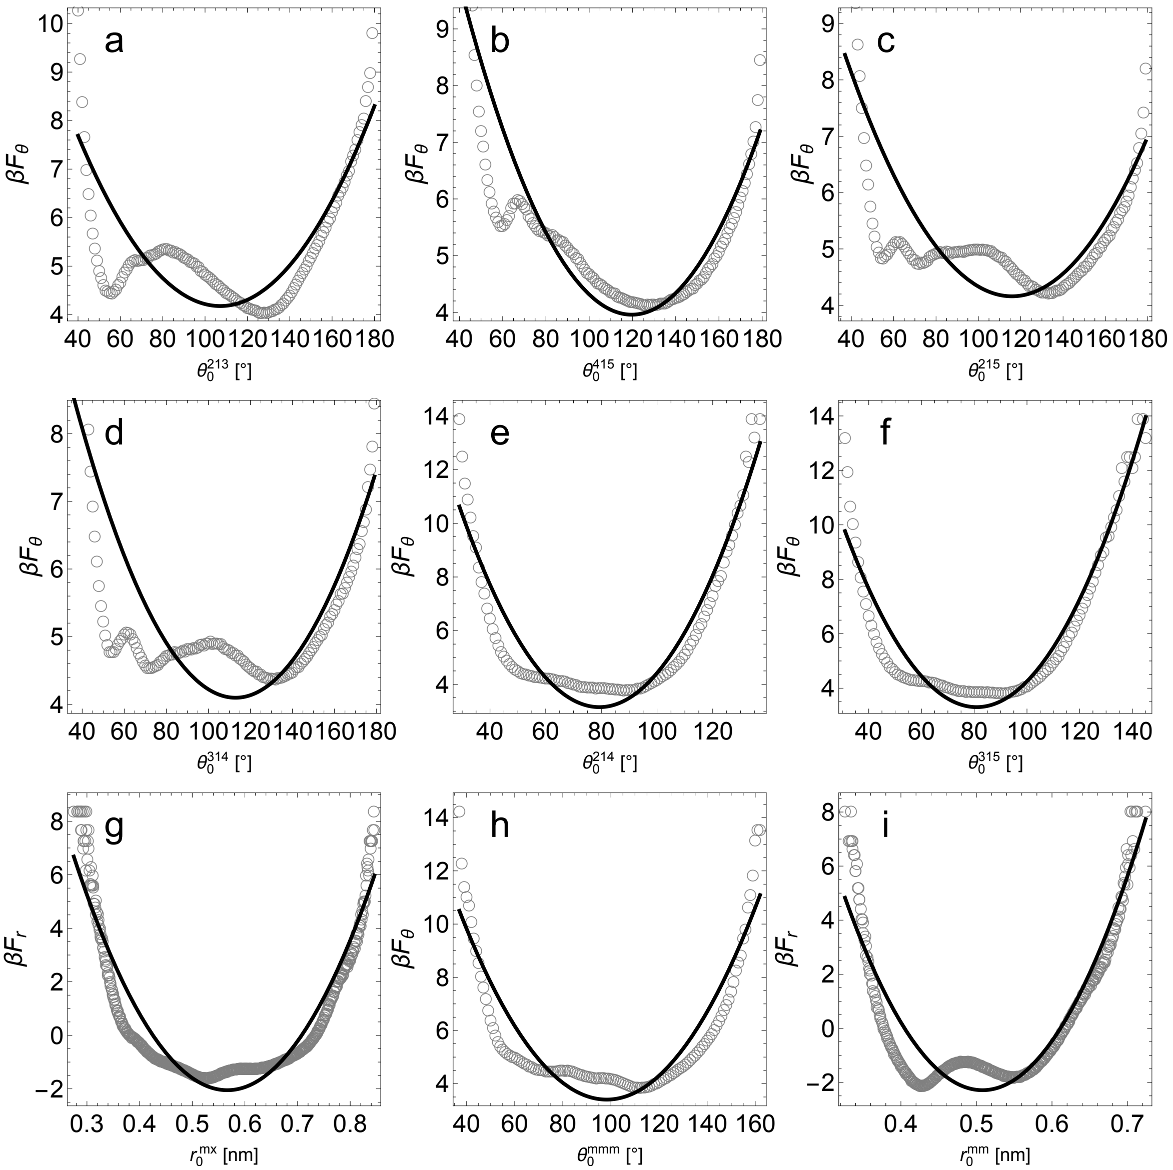


FIG. S12. Free energies (symbols) obtained from the all-atom simulations and fitted harmonic potentials (solid curves) given by eqns S8 and S9. See text for details.

energy $F_r^{\rm mx}$ between CG PNIPAM–BIS monomers is shown in Fig. S12g. The bending $F_\theta^{\rm mmm}$ and the stretching $F_r^{\rm mm}$ free energies in CG PNIPAM monomers are shown in Figs. S12h and i, respectively. We compared all the simulation data with the harmonic potentials in eqns S8 and S9, and determined the bond parameters as shown in Table S3. The thermal energy $k_{\rm B}T$ and the LJ length $\sigma = 0.4$ nm were used as respective units.

TABLE S3. Bond parameters in eqns S8 and S9, determined by fitting to all-atom simulation data shown in Fig. S12.

| complementary pair | 2-1-3 4-1-5 | 2-1-5 3-1-4 | 2-1-4 3-1-5 |
|---|---|---|---|
| $K_\theta^{\rm mxm}/k_{\rm B}T$ | $8.5 \times 10^{-4}$ | $7.2 \times 10^{-4}$ | $2.8 \times 10^{-3}$ |
| $\theta_0^{\rm mxm}$/deg | 113.4 | 114.4 | 80.1 |
| $K_r^{\rm mx}/(k_{\rm B}T/\sigma^2)$ | 16.4 | | |
| $r_0^{\rm mx}/\sigma$ | 1.4 | | |
| $K_\theta^{\rm mmm}/k_{\rm B}T$ | $1.9 \times 10^{-3}$ | | |
| $\theta_0^{\rm mmm}$/deg | 98.2 | | |
| $K_r^{\rm mm}/(k_{\rm B}T/\sigma^2)$ | 34.4 | | |
| $r_0^{\rm mm}/\sigma$ | 1.3 | | |


[1] J. Shin, A. G. Cherstvy, W. K. Kim, and V. Zaburdaev, Phys. Chem. Chem. Phys. **19**, 18338 (2017).
[2] W. K. Kim, A. Moncho-Jordá, R. Roa, M. Kanduč, and J. Dzubiella, Macromolecules **50**, 6227 (2017).
[3] H. Yasuda, C. Lamaze, and L. D. Ikenberry, Die Makromol. Chemie **118**, 19 (1968).
[4] H. Yasuda, L. Ikenberry, and C. Lamaze, Die Makromol. Chemie **125**, 108 (1969).
[5] H. Yasuda, A. Peterlin, C. Colton, K. Smith, and E. Merrill, Die Makromol. Chemie **126**, 177 (1969).
[6] N. A. Peppas and C. T. Reinhart, J. Memb. Sci. **15**, 275 (1983).
[7] C. T. Reinhart and N. A. Peppas, J. Memb. Sci. **18**, 227 (1984).
[8] S. R. Lustig and N. A. Peppas, J. Appl. Polym. Sci. **36**, 735 (1988).
[9] B. Amsden, Macromolecules **31**, 8382 (1998).
[10] D. S. Clague and R. J. Phillips, Phys. Fluids **8**, 1720 (1996).
[11] J.-M. Petit, B. Roux, X. Zhu, and P. Macdonald, Macromolecules **29**, 6031 (1996).
[12] L. Masaro and X. Zhu, Prog. Polym. Sci. **24**, 731 (1999).
[13] T. E. Andreoli and J. A. Schafer, *Principles of water and nonelectrolyte transport across membranes* (Springer, 1980).
[14] S. Milster, R. Chudoba, M. Kanduč, and J. Dzubiella, Phys. Chem. Chem. Phys. **21**, 6588 (2019).
[15] V. Palivec, D. Zadrazil, and J. Heyda, arXiv e-prints arXiv:1806.05592 (2018), 1806.05592.
[16] B. Hess, H. Bekker, H. J. C. Berendsen, and J. G. E. M. Fraaije, Journal of Computational Chemistry **18**, 1463 (1997).
[17] U. Essmann, L. Perera, M. L. Berkowitz, T. Darden, H. Lee, and L. G. Pedersen, J. Chem. Phys. **103**, 8577 (1995).
[18] G. Bussi, D. Donadio, and M. Parrinello, J. Chem. Phys. **126**, 14101 (2007).
[19] H. J. C. Berendsen, J. P. M. Postma, W. F. van Gunsteren, A. DiNola, and J. R. Haak, J. Chem. Phys. **81**, 3684 (1984).
